# Supplementary material for: Fluctuation-induced acceleration of inter-ligand exciton transfer in bis(dipyrrinato)Zn(II) complex
Source: arXiv:2602.16617 ancillary file (2026-04-17)
Supplement: Supplementary file 1 [file si.pdf]

**Supporting Information: Fluctuation-induced acceleration of inter-ligand exciton transfer in bis(dipyrrinato)Zn(II) complex**

Hiroki Uratani[1,2] and Hirofumi Sato[1,3]

[1)] *Department of Molecular Engineering, Graduate School of Engineering, Kyoto University, Kyoto, 615-0510, Japan*

[2)] *PRESTO, Japan Science and Technology Agency, Kawaguchi, Saitama, 332-0012, Japan*[a)]

[3)] *Fukui Institute for Fundamental Chemistry, Kyoto University, Kyoto, 606-8103, Japan*

[a)] Electronic mail: uratani@moleng.kyoto-u.ac.jp

## S1. NATURAL TRANSITION ORBITALS FOR LOW-LYING EXCITED STATES OF ZN(DP)$_2$

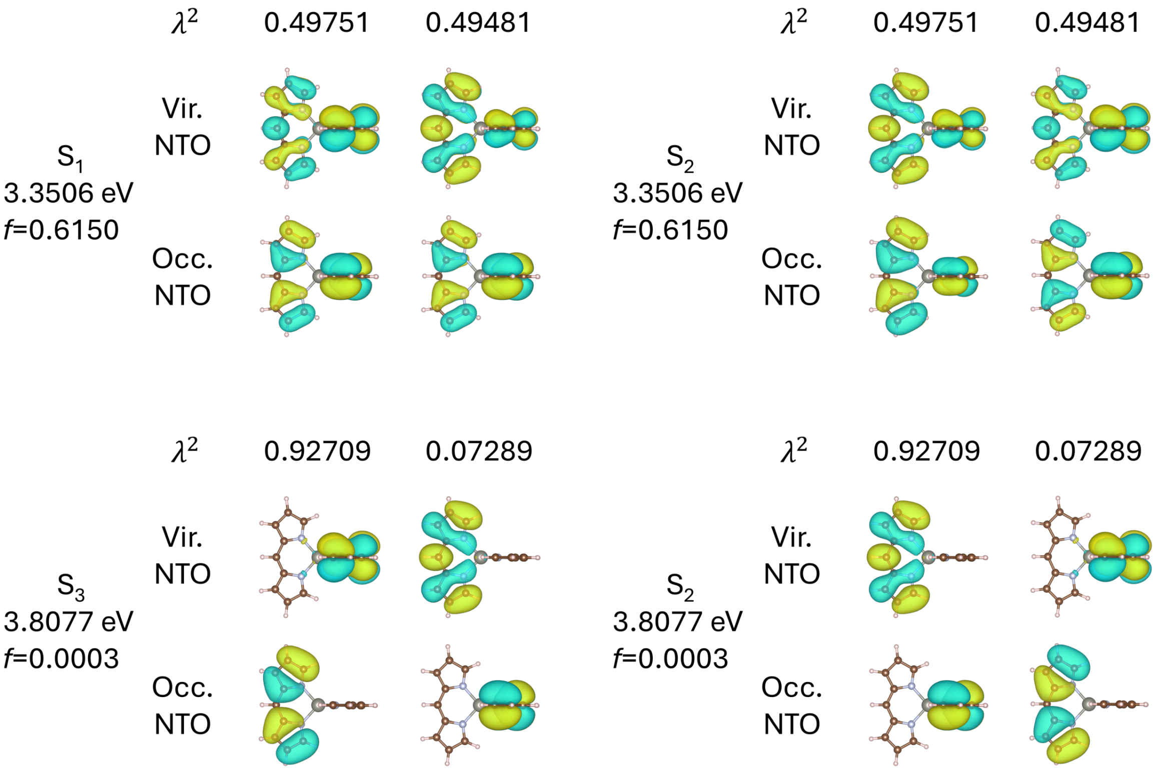


FIG. S1. NTOs for $S_1$–$S_4$ states of Zn(dp)$_2$ at the $S_0$ stable geometry (isolevel=0.015). The squared singular value ($\lambda^2$) is also shown for each occupied–virtual NTO pair. Note that ($S_1$, $S_2$) and ($S_3$, $S_4$) are degenerated pairs, so the wavefunctions have arbitrariness subject to unitary transformation within the two-state spaces.

## S2. DEFINITION OF DIHEDRAL ANGLE BETWEEN TWO DPS

The dihedral angle between the two dps in $Zn(dp)_2$ is defined as follows. The vector sets that span the dp1 plane ($\mathbf{v}^1_{\mathrm{dp1}}$ and $\mathbf{v}^2_{\mathrm{dp1}}$) and that span the dp2 plane ($\mathbf{v}^1_{\mathrm{dp2}}$ and $\mathbf{v}^2_{\mathrm{dp2}}$) are defined as shown in Figure S2. Then, the vectors $\mathbf{n}_{\mathrm{dp1}}$ and $\mathbf{n}_{\mathrm{dp2}}$, which are normal to dp1 and dp2 planes, respectively, are defined as

$$\mathbf{n}_{\mathrm{dp1}} = \mathbf{v}^1_{\mathrm{dp1}} \times \mathbf{v}^2_{\mathrm{dp1}} \tag{S1}$$

$$\mathbf{n}_{\mathrm{dp2}} = \mathbf{v}^1_{\mathrm{dp2}} \times \mathbf{v}^2_{\mathrm{dp2}} \tag{S2}$$

Finally, the dihedral angle $\phi$ is calculated as

$$\phi = \arccos\left(\frac{\mathbf{n}_{\mathrm{dp1}} \cdot \mathbf{n}_{\mathrm{dp2}}}{\left|\mathbf{n}_{\mathrm{dp1}}\right| \left|\mathbf{n}_{\mathrm{dp2}}\right|}\right) \tag{S3}$$

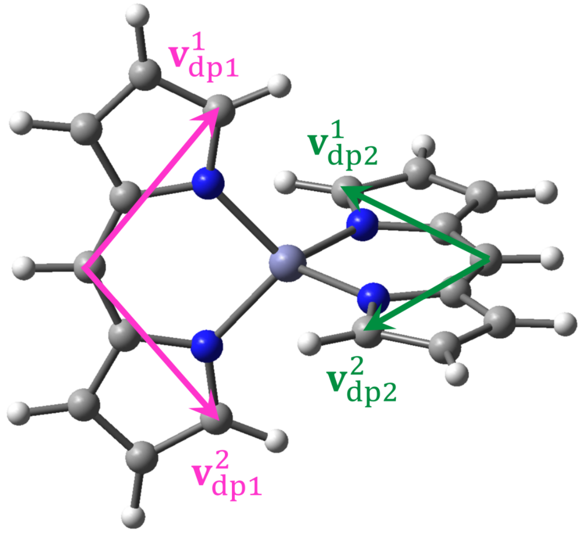


FIG. S2. Definition of vectors $\mathbf{v}^1_{\mathrm{dp1}}$, $\mathbf{v}^2_{\mathrm{dp1}}$, $\mathbf{v}^1_{\mathrm{dp2}}$, and $\mathbf{v}^2_{\mathrm{dp2}}$. The both ends of each magenta or green arrow are located on carbon atoms. White, gray, blue, and silver spheres represent H, C, N, and Zn atoms, respectively.

## S3. PROCEDURE FOR CALCULATION OF MONOMER EXCITATION ENERGIES

For each snapshot taken from the NA-MD trajectories, the monomer (here taken as dp1, but the same applies to dp2 except the permutation of labels), excitation energies were calculated in the following procedure. The geometry for the monomer calculations was constructed by dp2 atoms except the two N atoms coordinated to Zn atom, and then substituting the N atoms with $NH_3$ and $Cl^-$ to preserve charge neutrality (Figure S3). $NH_3$ was placed such that the position of N atom in $NH_3$ is the same with that of the N atom in dp2 to be substituted. The $NH_3$ was oriented such that the total vector of three N→H vectors is aligned to the Zn–N bond. The position of $Cl^-$ was determined such that the resulting Zn–Cl bond length is 2.24 Å and Zn–Cl vector is aligned to the original Zn–N bond, where N is to be substituted. Two different geometries can be constructed because there are two N atoms to be substituted, one with $NH_3$ and the other one with $Cl^-$, where the ordering is arbitrary. Hence, the monomer excitation energies were calculated for these two geometries and the averaged value was used for the subsequent analyses. The excitation energies were calculated at TD-CAM-B3LYP/Def2SV(P) level of theory as implemented in Gaussian 16 program package, which is the same quantum-chemical calculation setting with that for the NA-MD simulations reported in the main text. The resulting $S_0 \rightarrow S_1$ excitation energies were taken as the monomer excitation energies.

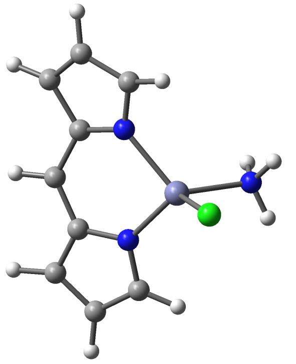

FIG. S3. An example of monomer geometry constructed from a NA-MD snapshot. White, gray, blue, silver, and green spheres represent H, C, N, Zn, and Cl, respectively.

## S4. NORMAL-MODE DECOMPOSITION OF $\bar{\mathbf{Q}}$

Figure S4 presents the weights of $S_0$ normal modes in $\bar{\mathbf{Q}}$, i.e., $\left(\bar{\mathbf{Q}} \cdot \mathbf{e}_m\right)^2$, where $\mathbf{e}_m$ denotes the displacement vector along the normal mode $m$. The calculation was conducted in the mass-weighted coordinate system. Figure S5 illustrates the displacement vectors of the dominant normal

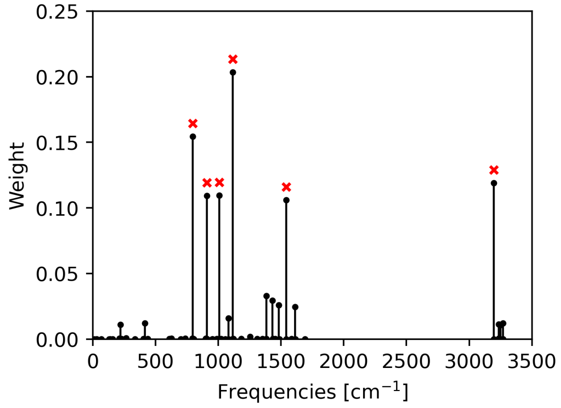


FIG. S4. Weights of $S_0$ normal modes in $\bar{\mathbf{Q}}$. Modes that have significant contribution (weight¿0.1) are indicated by red cross marks.

modes (indicated by red cross marks in Figure S4).

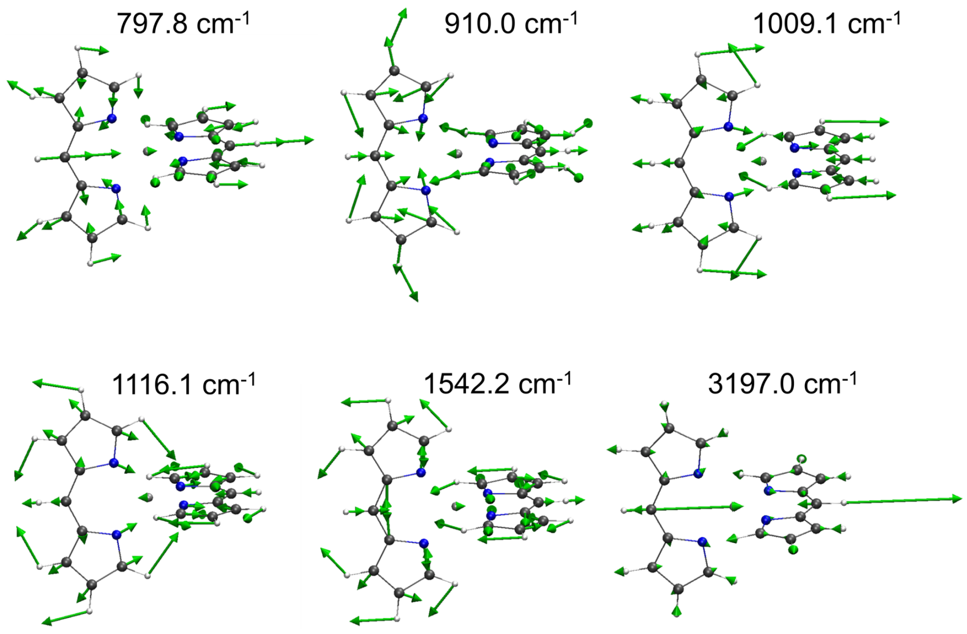


FIG. S5. Displacement vectors of dominant component normal modes in $\bar{\mathbf{Q}}$.

## S5. REGRESSION ANALYSIS USING THE $S_1$ STABLE GEOMETRY AS ORIGIN

In parallel to the definition of reaction coordinate $Q$, in which the origin is the $S_0$ stable geometry, the alternative reaction coordinate $Q^{S_1}$, in which the origin is the $S_1$ stable geometry, is defined through the linear regression analysis in analogy of eq. 14 in the main text. The corresponding numerical results are shown in Figure S6.

$$\Delta E^{(i)}_{\mathrm{Pred}} = a\bar{\mathbf{q}} \cdot \left(\mathbf{R}^{(i)} - \mathbf{R}^{S_1}_0\right) + b \tag{S4}$$

$$\bar{\mathbf{Q}}^{S_1}, A, B = \underset{\bar{\mathbf{q}},a,b}{\mathrm{argmin}} \sum_i \left|\Delta E^{(i)}_{\mathrm{Pred}}(\bar{\mathbf{q}}, a, b) - \Delta E^{(i)}\right|^2 \tag{S5}$$

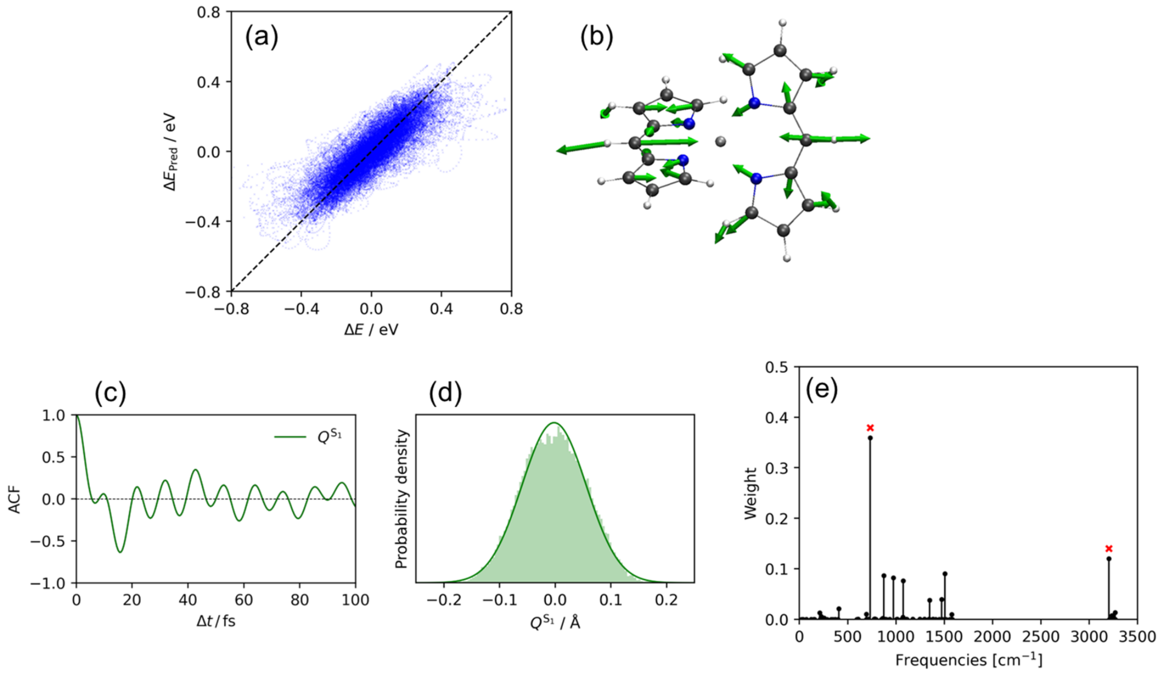


FIG. S6. (a) Comparison of the diabatic energy gaps obtained from the "monomer" TD-DFT calculations ($\Delta E$ :), and those predicted from the linear regression model using the $S_1$ stable geometry as origin ($\Delta E_{\mathrm{Pred}}$). (b) Atomic displacement vector in the direction of $\bar{\mathbf{Q}}^{S_1}$ (green arrows). (c) VACF for $Q^{S_1}$. (d) Distribution of $Q^{S_1}$ sampled from the NA-MD trajectories. (e) Weights of $S_1$ normal modes in $\bar{\mathbf{Q}}^{S_1}$. Modes that have significant contribution (weight>0.1) are indicated by red cross marks.

## S6. GROUND-STATE DYNAMICS

Figure S7 indicates the VACFs of $\phi$ and $Q$ obtained from the ground-state (GS) Born–Oppenheimer molecular dynamics started from the same initial geometries and momenta with the NA-MD simulations. Fugure S8 shows the distribution of $\phi$ and $Q$ sampled from the same trajectories.

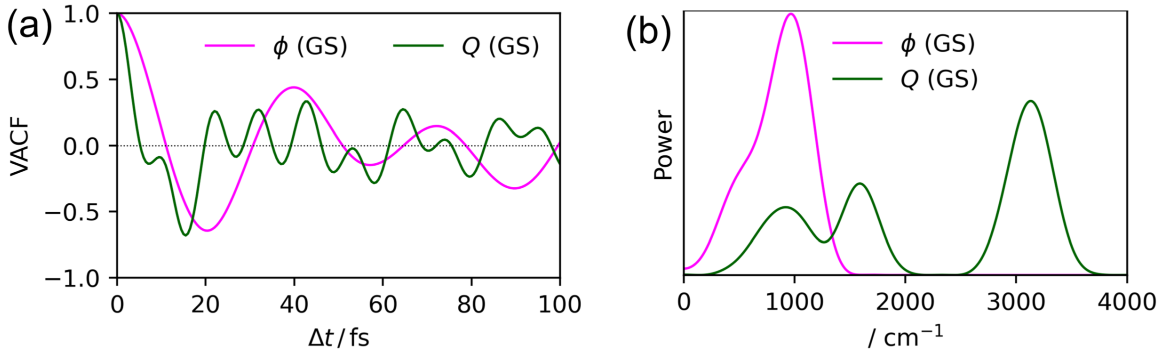


FIG. S7. (a) VACFs for the dihedral angle ($\phi$) and the reaction coordinate ($Q$) obtained from the GS trajectories. (b) Power spectra of VACFs.

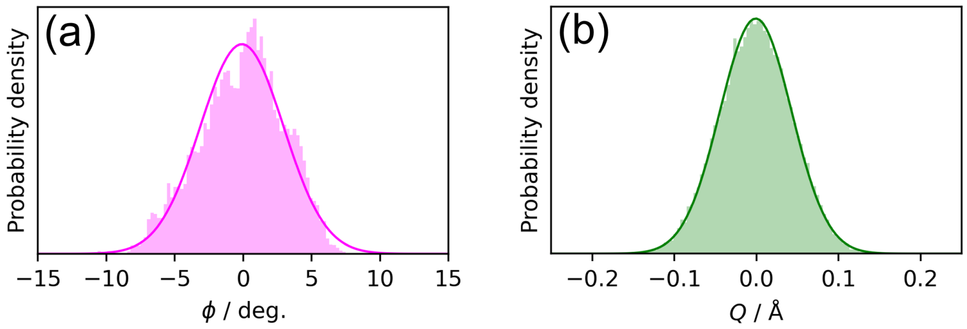


FIG. S8. Distribution of (a) $\phi$ and (b) $Q$ sampled from the GS trajectories.
